# Supplementary material for: Optimal management of a stochastically varying population when policy adjustment is costly
Source: arXiv:1507.07037 source file (2015-07-24)
Supplement: Supplementary file 1 [file supplement.pdf]

# Supplement to: Optimal management of a stochastically varying population when policy adjustment is costly

Carl Boettiger*[a], Michael Bode[c], James N. Sanchirico[b], Jacob LaRiviere[e], Alan Hastings[b], Paul R. Armsworth[d]

[a] *Department of Environmental Science, Policy and Management, University of California, Berkeley, 130 Mulford Hall #3114, Berkeley, CA 94720-3114, USA*

[b] *Department of Environmental Science and Policy, University of California, Davis*

[c] *School of Botany, University of Melbourne, Australia*

[d] *Department of Ecology and Evolutionary Biology, University of Tennessee, Knoxville*

[e] *Department of Economics, University of Tennessee, Knoxville*

## Abstract

## Supplementary material

### *Code and data for methods and analysis*

All code and data used in this analysis can be found under the project's GitHub repository: https://github.com/cboettig/pdg_control. A snapshot of this repository representing the precise versions of the code used in this analysis has been permanently archived in the scientific software and data repository Zenodo, managed by CERN; and should be referenced or cited using its assigned digital object identifier, doi:10.5281/zenodo.21416 (This DOI is also clearly linked from the GitHub repository).

### *Organization of code*

The project repository is organized as an R package. The intent is not to provide a general-purpose software tool for this kind of analysis, but rather to rely on a standardized directory structure for representing complex projects. It is our hope that this facilities understanding, reproducibility, and further exploration of these results sensu Gentleman & Temple Lang 2004, but caution that additional software engineering would be required before

*Corresponding author
*Email address:* `cboettig (at) berkeley.edu` (Carl Boettiger)

any of this could be applied in a different context. The functions provided are largely specific to the analyses presented here and may undocumented or incompletely documented.

The source documents for both the manuscript and supplement are also found in the code repository using the dynamic document `.Rmd` format which embeds all of the code required for the analysis; see http://rmarkdown.rstudio.com/.

Within the `.Rmd` files themselves are found only the blocks of code required to generate each of the figures shown in the manuscript. The analysis is sourced in from an external R script, `analysis.R` by a code block at the beginning of the `.Rmd` file. This script in turn relies on more modular functions defined in the `R/` directory that define the stochastic dynamic programming optimization algorithms, simulation routines, and so forth.

### *Data*

All empirical or simulated data shown in the figures can also be found as tabular `.csv` files in this repository.

### *Dependencies and machine images*

The package DESCRIPTION file lists the software dependencies required to run the included scripts. To facilitate portability and preservation of these dependencies, we also provide a machine image with all the necessary dependencies already installed which can be run on most common computer platforms using Docker. Our Docker image, `cboettig/pdg-control` can be freely downloaded from the Docker Hub, or built using the Dockerfile included in the package repository.

### *Impact on the stock dynamics*

Figure S1 shows the corresponding stock dynamics for the replicates illustrated in Figure 3 of the main text. The impact of the adjustment cost on the stock dynamics is less dramatic than it is on the harvest dynamics, due to the stochastic growth in stock sizes and the sequence in which the steps are applied: stock values are assessed without error, then an optimal harvest is determined (using the pre-computed optimal policy based on both the stock assessment and the

previous harvest, to account for possible adjustment costs), and then the stock that escapes harvesting recruits stochastically to set the population size for the next year.

Though this results in an effect that is less pronounced, the stock dynamics of Figure S1 reflect the same general trends observed in Main text Figure 3; e.g. the fixed fee $\Pi_3$ results in the most exaggerated fluctuations in the stock sizes. It is worth noting how changes in policy costs alone, such as introducing or rising fixed costs, can have important knock-on effects to population dynamics such as increased variance, a recent phenomenon observed in important fisheries that has received much attention elsewhere (Anderson et al. 2008).

Recall that in our model definition, stock sizes are measured before harvest ($h_t$ being determined after observing stock size $N_t$) and thus show less influence of the policy cost than the harvest itself.

Figure S2 shows the same summary statistics illustrating the trends of increasing adjustment costs on the *stock* dynamics, instead of the *harvest* dynamics shown in Figure 4 of the main text. Note that the variance in stock sizes under the quadratic penalty ($\Pi_2$) increases, while in Figure 4 of the main text the corresponding variance in the harvest decreases. Under costly adjustment, the undershooting behavior of the $\Pi_2$ harvest policy cannot absorb as much of the natural fluctuation, resulting in increased variation in the stock sizes.

*Additional stochastic realizations*

Figure 3 of the main text shows only a single stochastic realization. Here in Figure S3 we provide a sample of further realizations (including both stock and harvest dynamics).

*Economic penalties using quadratic costs*

Figure S4 shows that adding quadratic terms to the cost of fishing effort directly, as in Lewis (1981) or McGough et al. (2009), results in a similar smoothing effect as we observe in quadratic adjustment costs ($\Pi_2$), which contrasts sharply with the patterns we observe in other functional forms. This case corresponds to a profit function defined as:

$$\Pi_4(N_t, h_t) = ph_t - c_0E_t - c_4E_t^2$$

Where $c_4$ is calibrated as in the case of the other coefficients to induce the fixed reduction of net present value relative to $NPV_0$.

Like the $\Pi_2$ adjustment cost based penalty, this quadratic cost based penalty shows periods of constant, strictly positive policy only 10.2% of the time, and exhibits the same kind of smoothing of more small adjustments that is seen in $\Pi_2$ scenario.

*Ignoring adjustment costs is worst than wrongly assuming adjustment costs*

Figure S5 extends Figure 5 of the main text across all three functional forms of adjustment costs, $\Pi_{1-3}$. To reduce over-plotting of Figure 5 we have also separated the distributions of dockside revenue and adjustment fees by scenario, such that the top row shows the distributions when the policy accounts for adjustment costs, and the bottom shows the policy when it does not (that is, the original Reed (1979) model applied to the scenario of costly adjustment).

Figure S6 extends the results shown in Figure 6 across different severities of adjustment cost, totaling from 10% up to 25% of the $NPV$ of the stock. While the same qualitative pattern is observed in all cases, it is strongest in the higher penalties.

*Mismatched penalty functions*

When policy costs are present, assuming the wrong functional form may or may not be worse than ignoring the presence of policy costs all together. Figure S7 considers several such cases. The X axis labels indicate first which policy is being used to drive the harvest decisions, and then which penalty is actually being applied. Thus $\Pi_1\_\Pi_2$ indicates a policy calculated under the linear ($\Pi_1$) costs, when the reality involves quadratic ($\Pi_2$) costs. Though the coefficients of the ($\Pi_2$) costs have been scaled such that the net effect is the same, the inferred policies differ. As a result, the value is slightly more than half of the optimal free solution when the expected reduction should only be 10% (panel A) less than optimal free based on the $c_i$ calibration. In this case, ignoring the costs all together is still worse than using $\Pi_1$ costs – the red bar is lower than the blue.

For fixed costs ($\Pi_3$), the reverse is true. Because fixed costs increase the volatility of the optimal solution while $\Pi_2$ costs decrease it, simply ignoring the cost of adjustment all together results in

a higher value than either assuming costs are quadratic ($\Pi_2$) when they are fixed ($\Pi_3$), or assuming they are fixed when they are quadratic. Scenarios in which true costs are quadratic (regardless of what cost structure is assumed by the policy) do significantly worse than those that are not (i.e. all cases that assume quadratic but actually have linear or fixed costs).

These patterns hold across the different size reductions shown (from 10% to 25%, Figure S8 panels a-d respectively), though net present value becomes negative under the quadratic form for the larger penalties as costs paid for adjustments exceed profits derived from harvest. (Though optimal solutions will always avoid negative net present values, these scenarios in which policies are applied under conditions other than assumed in the optimality calculation have no such guarantee.) For each scenario, results are averaged over 100 replicates.

*Robustness to reduction level*

Figures S8-S11 illustrate that the these qualitative patterns still hold at when the models are calibrated to a reduction in NPV of 10% or 30%, though naturally the magnitude of the pattern is greater when the penalty is larger (e.g. 30% vs 10%).

Anderson, C. N. K., C.-h. Hsieh, S. a Sandin, R. Hewitt, A. Hollowed, J. Beddington, R. M. May, and G. Sugihara. 2008. Why fishing magnifies fluctuations in fish abundance. Nature 452:835–9.

Lewis, T. R. 1981. Exploitation of a renewable resource under uncertainty. The Canadian Journal of Economics 14:422.

McGough, B., P. A. J., and C. Costello. 2009. Optimally managing a stochastic renewable resource under general economic conditions. The B.E. Journal of Economic Analysis & Policy 9:1–31.

Reed, W. J. 1979. Optimal escapement levels in stochastic and deterministic harvesting models. Journal of Environmental Economics and Management 6:350–363.

## List of Figures

S1 Example realization of optimal fish stock sizes under the different functional forms of adjustment costs, under the harvest policy dynamics shown in Figure 3 of the main text. . . . . . . . . . . . . . . . . . . . . . . . . . . . . . . . . . . . . 7

S2 Variance and autocorrelation of stock dynamics, as a function of the penalty coefficient. Adjustment penalty is calculated as percentage of the maximum expected $NPV$ in the basic case with no policy adjustment costs. . . . . . . . . 8

S3 Multiple realizations of optimal harvesting strategy and resulting fish stock sizes under the different functional forms of adjustment costs. . . . . . . . . . . . . . 9

S4 Quadratic costs to fishing effort show a similar pattern of smoothing to that which we observe in the quadratic adjustment cost model. . . . . . . . . . . . . . . . . . 10

S5 Distribution of profits from fishing and costs paid to adjustment. Distributions are shown when managing a system in which the adjustment costs present are determined by the model indicated, and compared to the same costs and profits of managing the same system using a Reed model, which ignores adjustment costs, and thus tends to pay much higher fees for adjustment. In contrast, the difference in profit after accounting for costs is only marginally less than the value derived by managing the population to optimize profits when ignoring adjustment costs (Reed model). . . . . . . . . . . . . . . . . . . . . . . . . . . . . . . . . . . . . 11

S6 Relative cost of ignoring adjustment costs when they are present ('ignoring', red) vs assuming the adjustment costs when they are absent ('assuming', blue), shown by penalty function over increasing magnitudes of cost. All values are relative to the cost-free adjustment optimum, NPV0. In each case, it is less costly to assume adjustment costs are present when they are not than it is to ignore them when they are present. The severity of the latter mistake increases sharply as adjustment costs make a larger fraction of the total costs. . . . . . . . . . . . . . 12

S7 Mismatches. X axis labels indicate the model used to derive the policy, followed by the model used to simulate the penalty. Blue bars show the net present value of that scenario. Compare to red bars, which show the consequence of using a policy that ignores costs all together in the same scenario (i.e. costs as indicated by second code), rather than assuming the policy indicated by the first code in the pair. All values are scaled to a fraction of the adjustment free net present value. 13

S8 Identical analysis to Figure 3 of the main text, but using a calibration corresponding to a 10% reduction in NPV. This results in a less pronounced version of the same qualitative pattern. . . . . . . . . . . . . . . . . . . . . . . . . . . . . . . . . . . 14

S9 Identical analysis to Figure 3 of the main text, but using a calibration corresponding to a 30% reduction in NPV. This results in a more pronounced version of the same qualitative pattern. . . . . . . . . . . . . . . . . . . . . . . . . . . . . . . . . . 15

S10 Results as in Figure 5 of the main text, but using a net reduction of NPV equal to 10%. . . . . . . . . . . . . . . . . . . . . . . . . . . . . . . . . . . . . . . . . 16

S11 Results as in Figure 5, but using a net reduction equal to 30% . . . . . . . . . . . 17

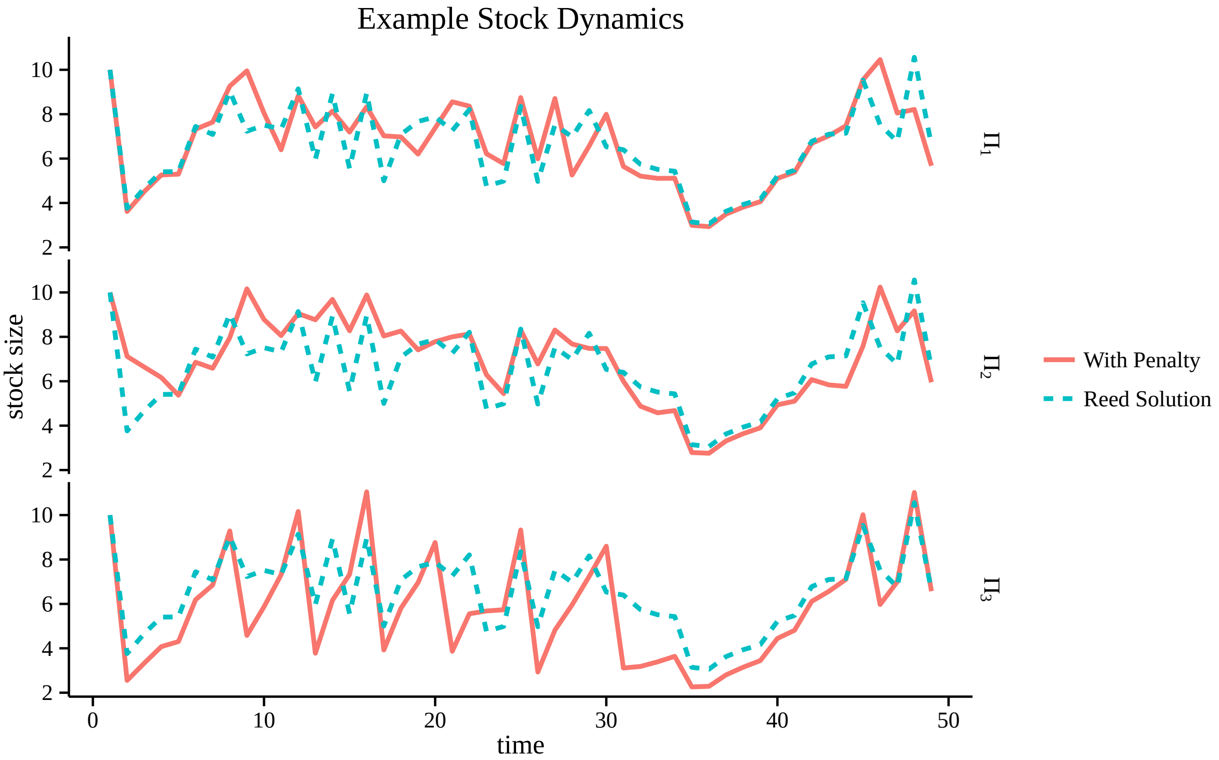


Figure S1: Example realization of optimal fish stock sizes under the different functional forms of adjustment costs, under the harvest policy dynamics shown in Figure 3 of the main text.

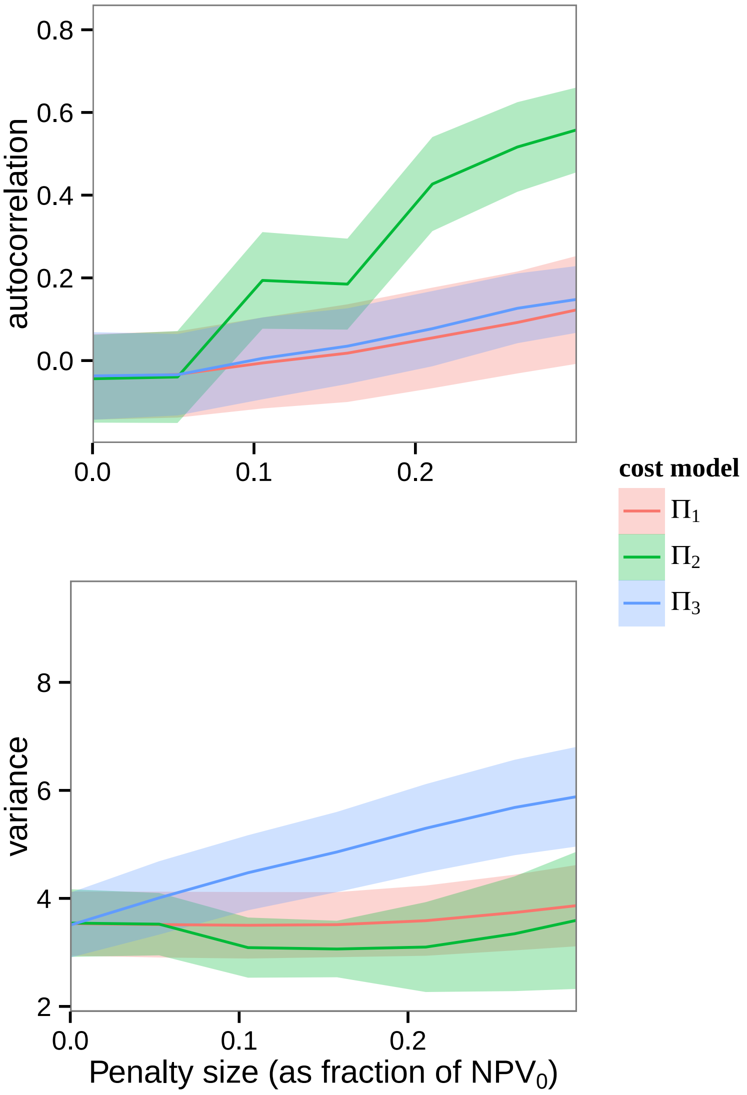


Figure S2: Variance and autocorrelation of stock dynamics, as a function of the penalty coefficient. Adjustment penalty is calculated as percentage of the maximum expected $NPV$ in the basic case with no policy adjustment costs.

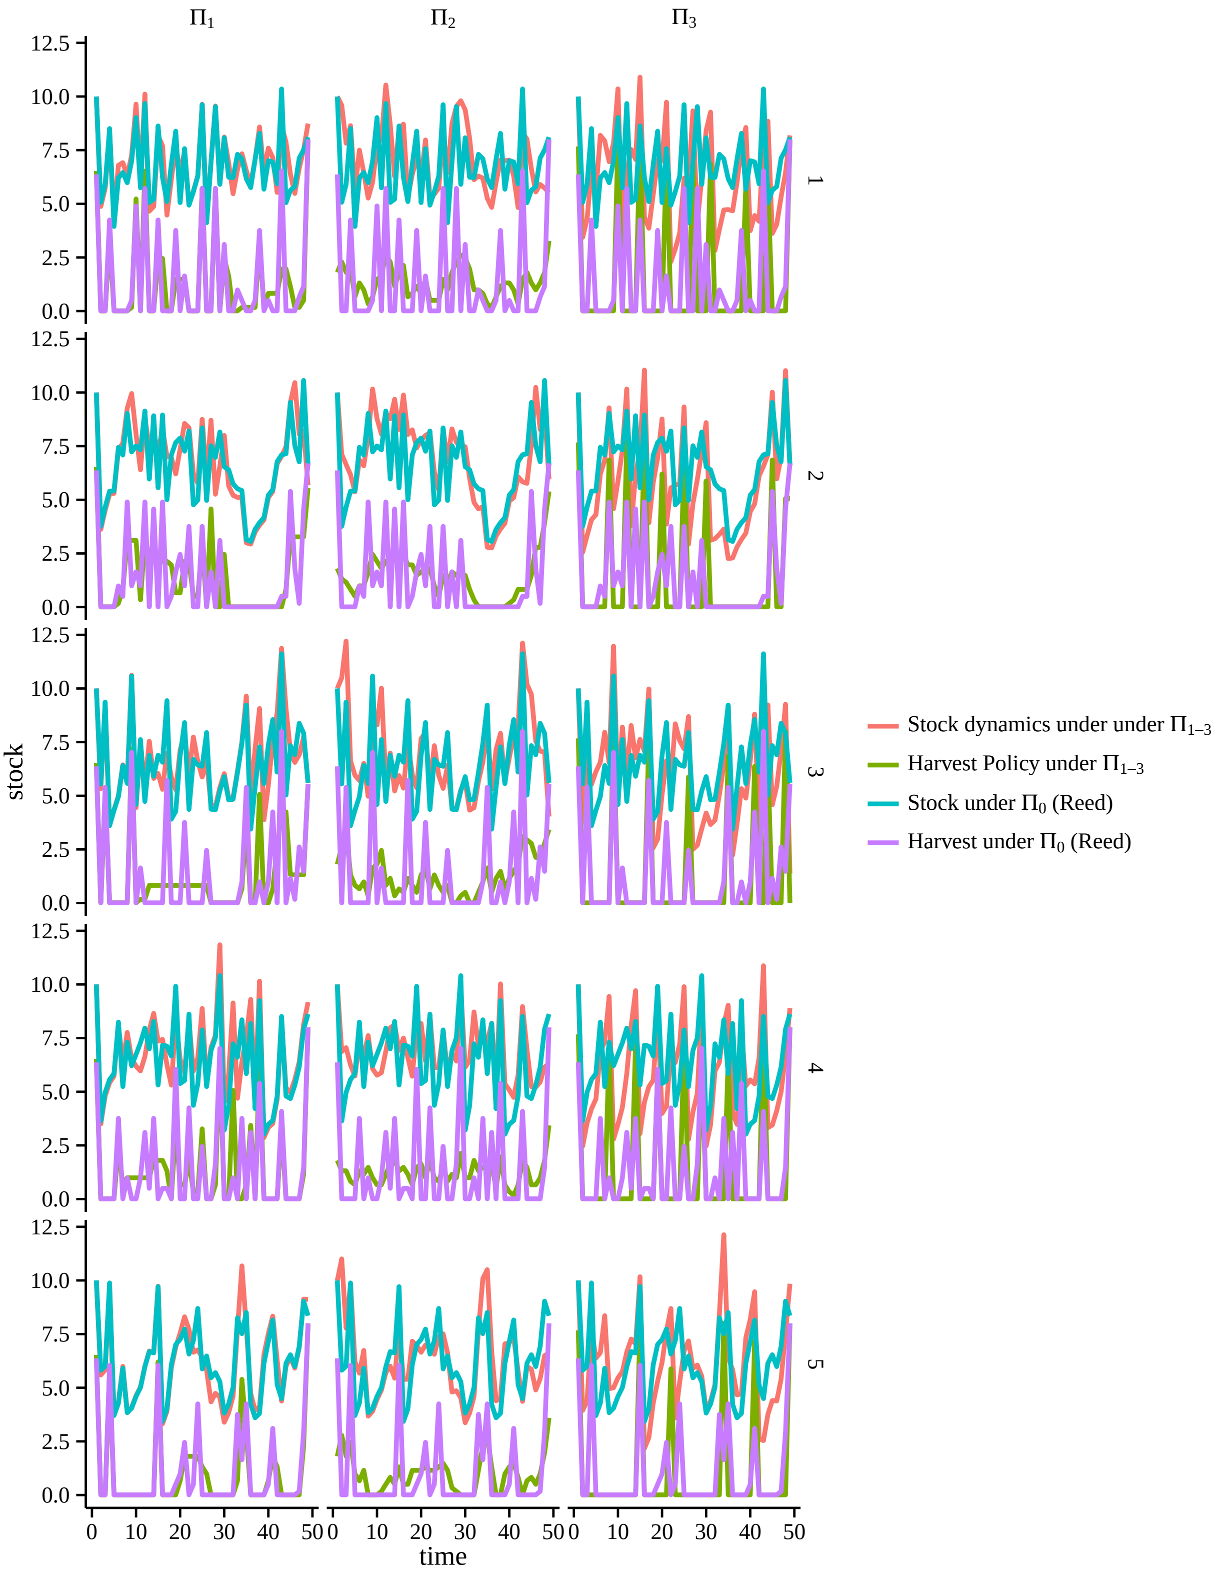


Figure S3: Multiple realizations of optimal harvesting strategy and resulting fish stock sizes under the different functional forms of adjustment costs.

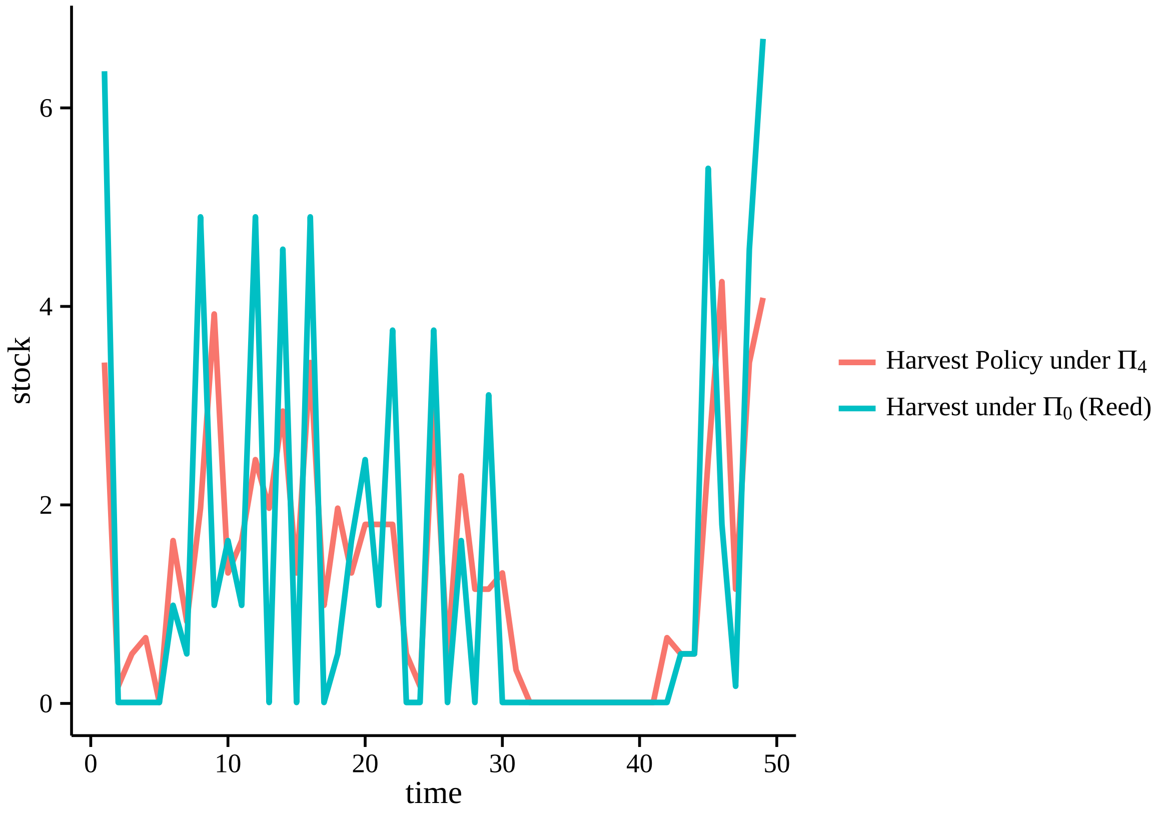


Figure S4: Quadratic costs to fishing effort show a similar pattern of smoothing to that which we observe in the quadratic adjustment cost model.

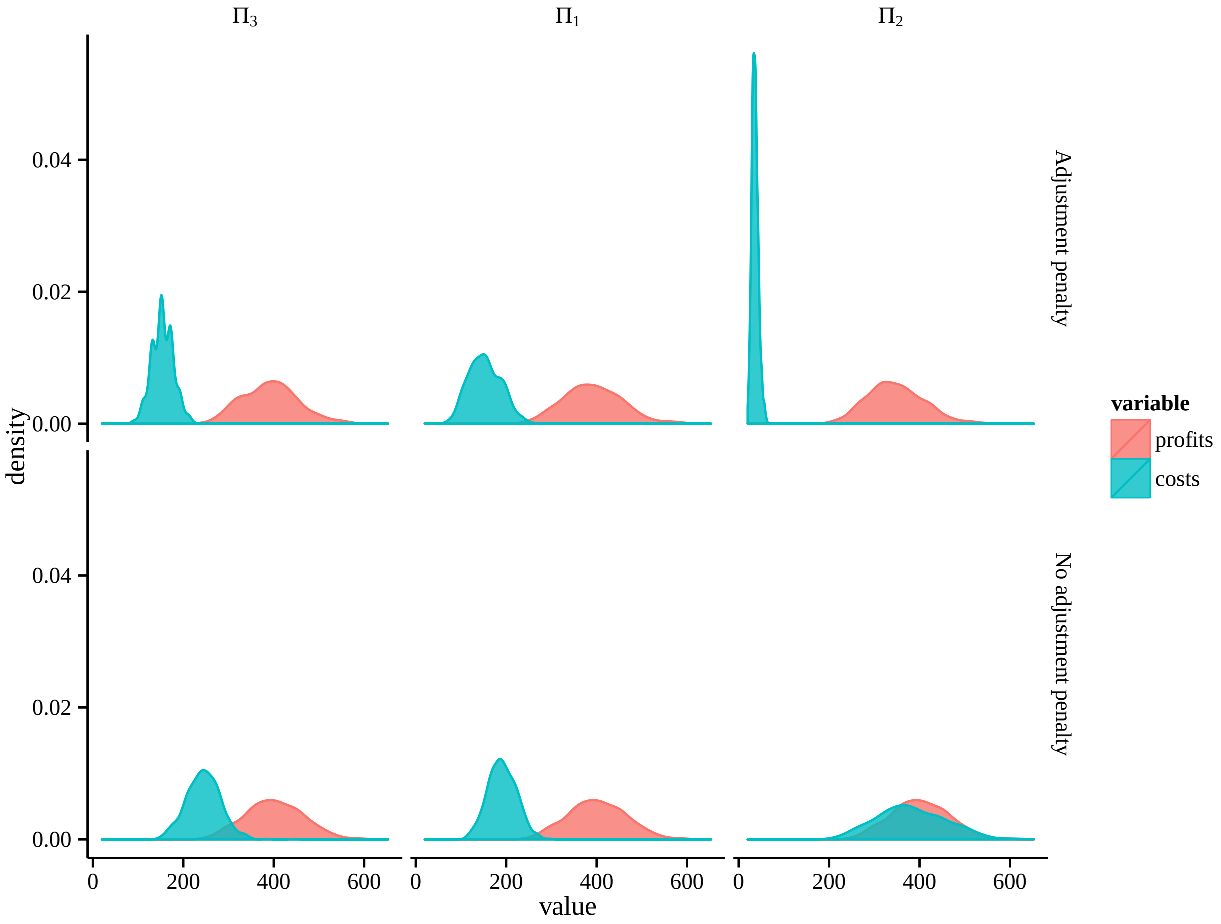


Figure S5: Distribution of profits from fishing and costs paid to adjustment. Distributions are shown when managing a system in which the adjustment costs present are determined by the model indicated, and compared to the same costs and profits of managing the same system using a Reed model, which ignores adjustment costs, and thus tends to pay much higher fees for adjustment. In contrast, the difference in profit after accounting for costs is only marginally less than the value derived by managing the population to optimize profits when ignoring adjustment costs (Reed model).

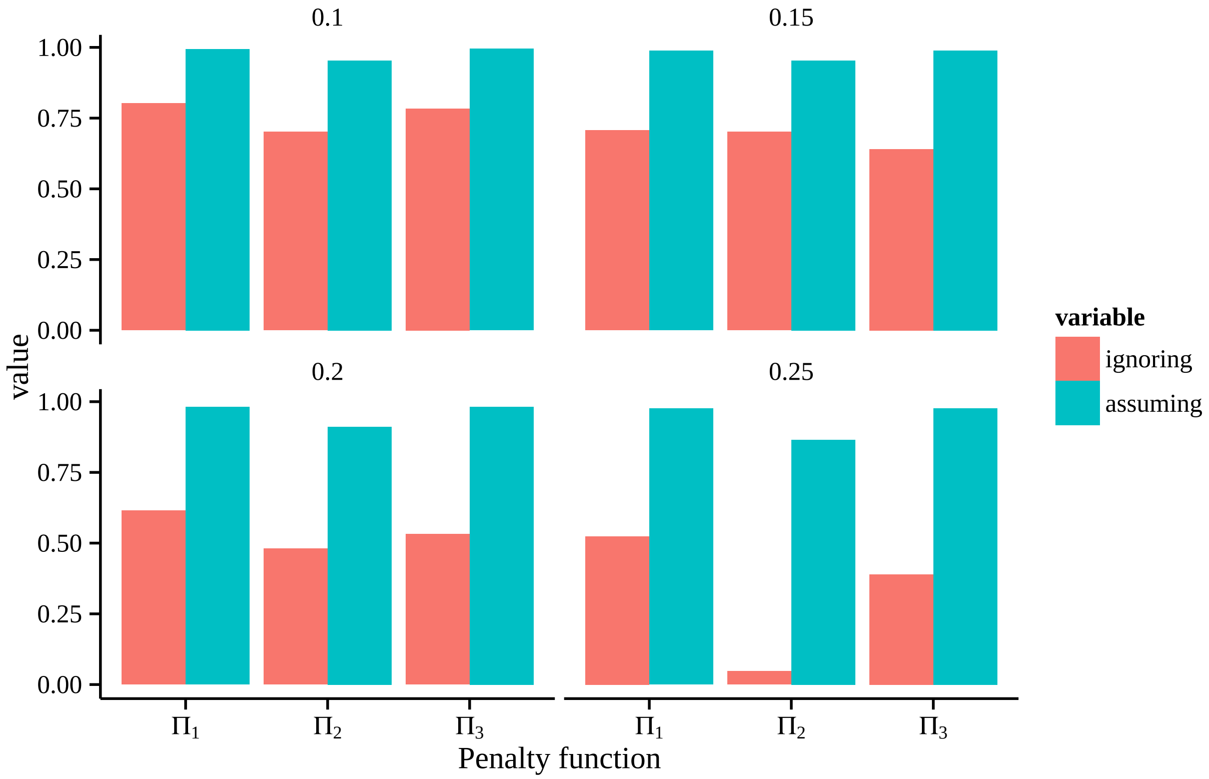


Figure S6: Relative cost of ignoring adjustment costs when they are present (‘ignoring’, red) vs assuming the adjustment costs when they are absent (‘assuming’, blue), shown by penalty function over increasing magnitudes of cost. All values are relative to the cost-free adjustment optimum, NPV0. In each case, it is less costly to assume adjustment costs are present when they are not than it is to ignore them when they are present. The severity of the latter mistake increases sharply as adjustment costs make a larger fraction of the total costs.

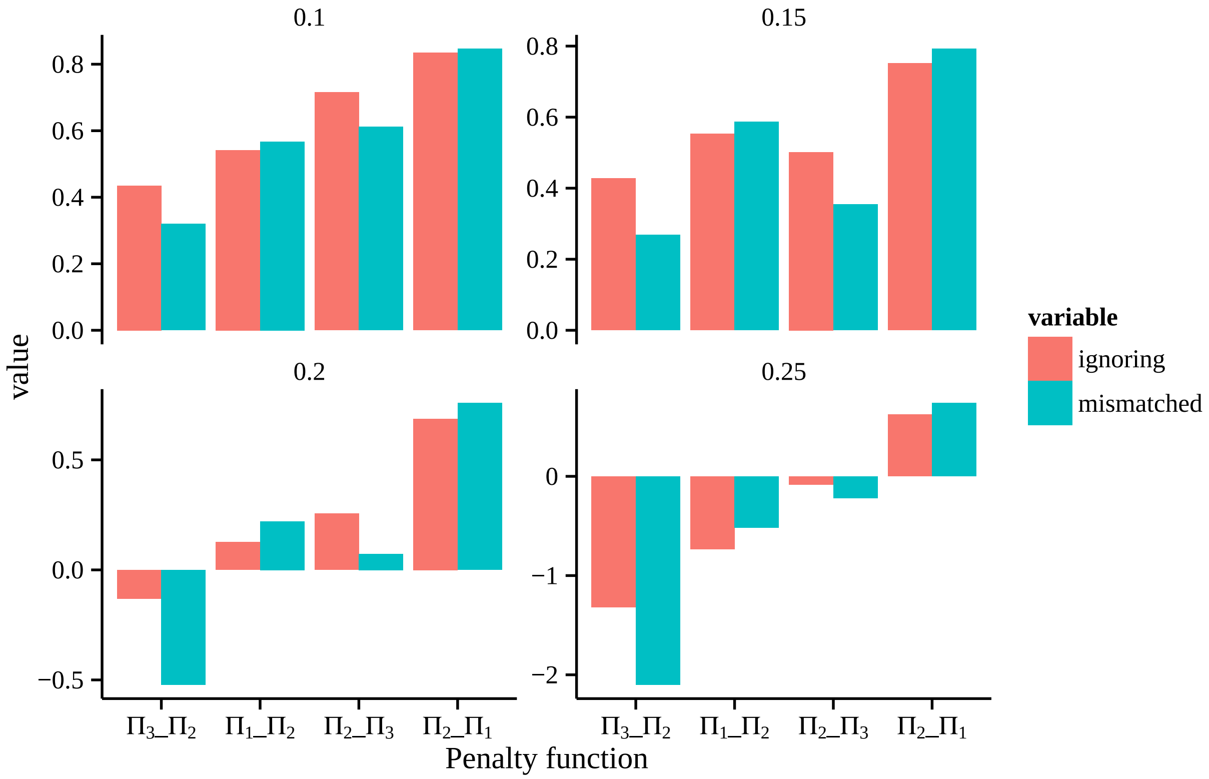


Figure S7: Mismatches. X axis labels indicate the model used to derive the policy, followed by the model used to simulate the penalty. Blue bars show the net present value of that scenario. Compare to red bars, which show the consequence of using a policy that ignores costs all together in the same scenario (i.e. costs as indicated by second code), rather than assuming the policy indicated by the first code in the pair. All values are scaled to a fraction of the adjustment free net present value.

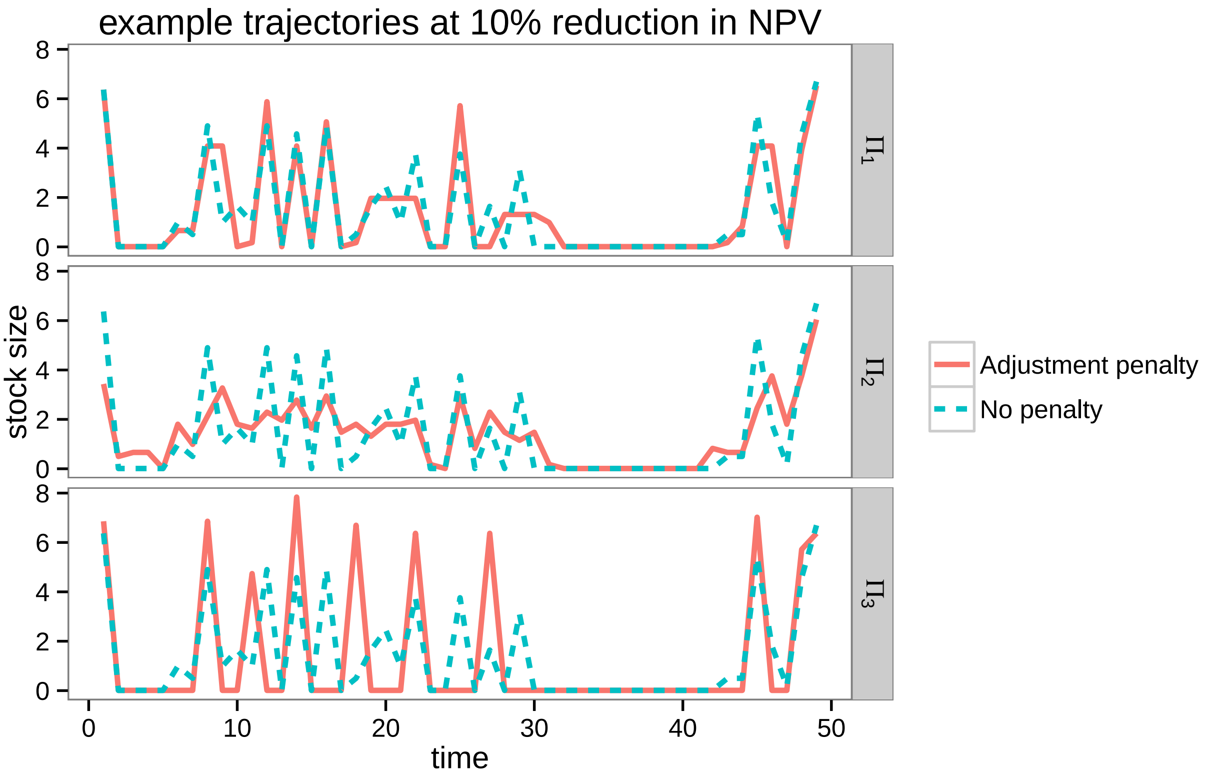


Figure S8: Identical analysis to Figure 3 of the main text, but using a calibration corresponding to a 10% reduction in NPV. This results in a less pronounced version of the same qualitative pattern.

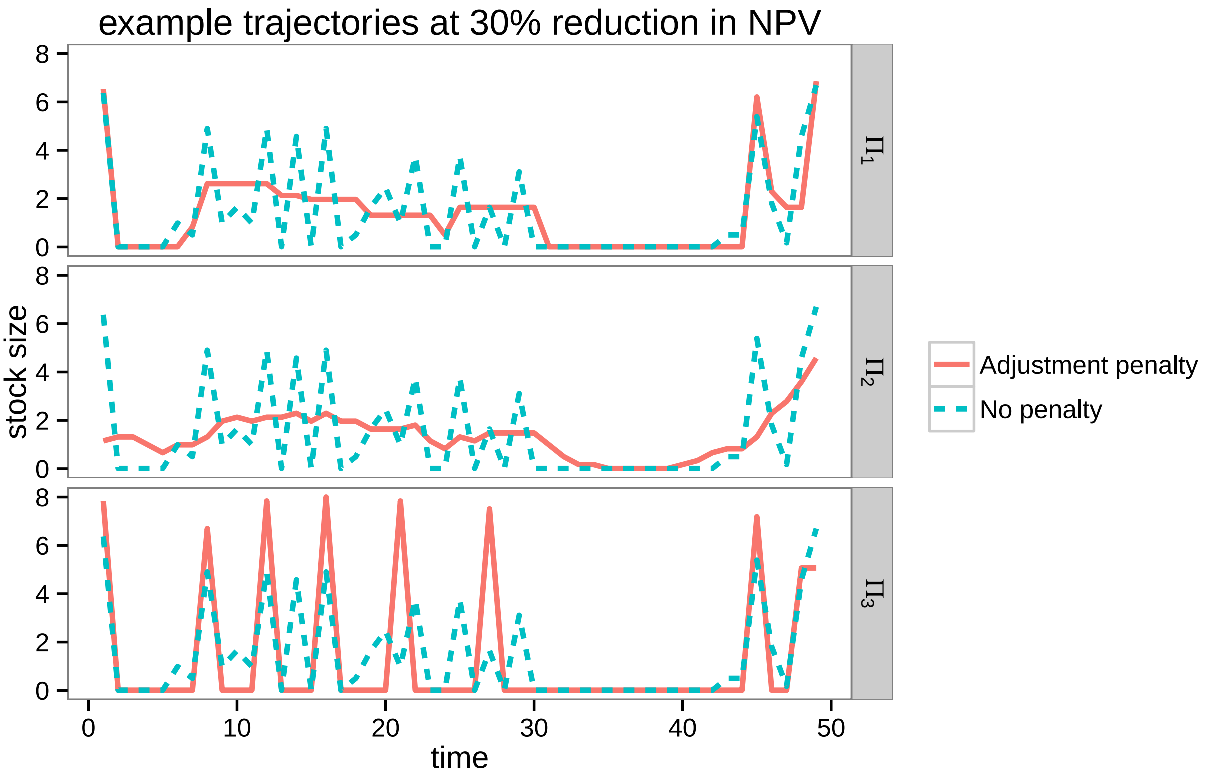


Figure S9: Identical analysis to Figure 3 of the main text, but using a calibration corresponding to a 30% reduction in NPV. This results in a more pronounced version of the same qualitative pattern.

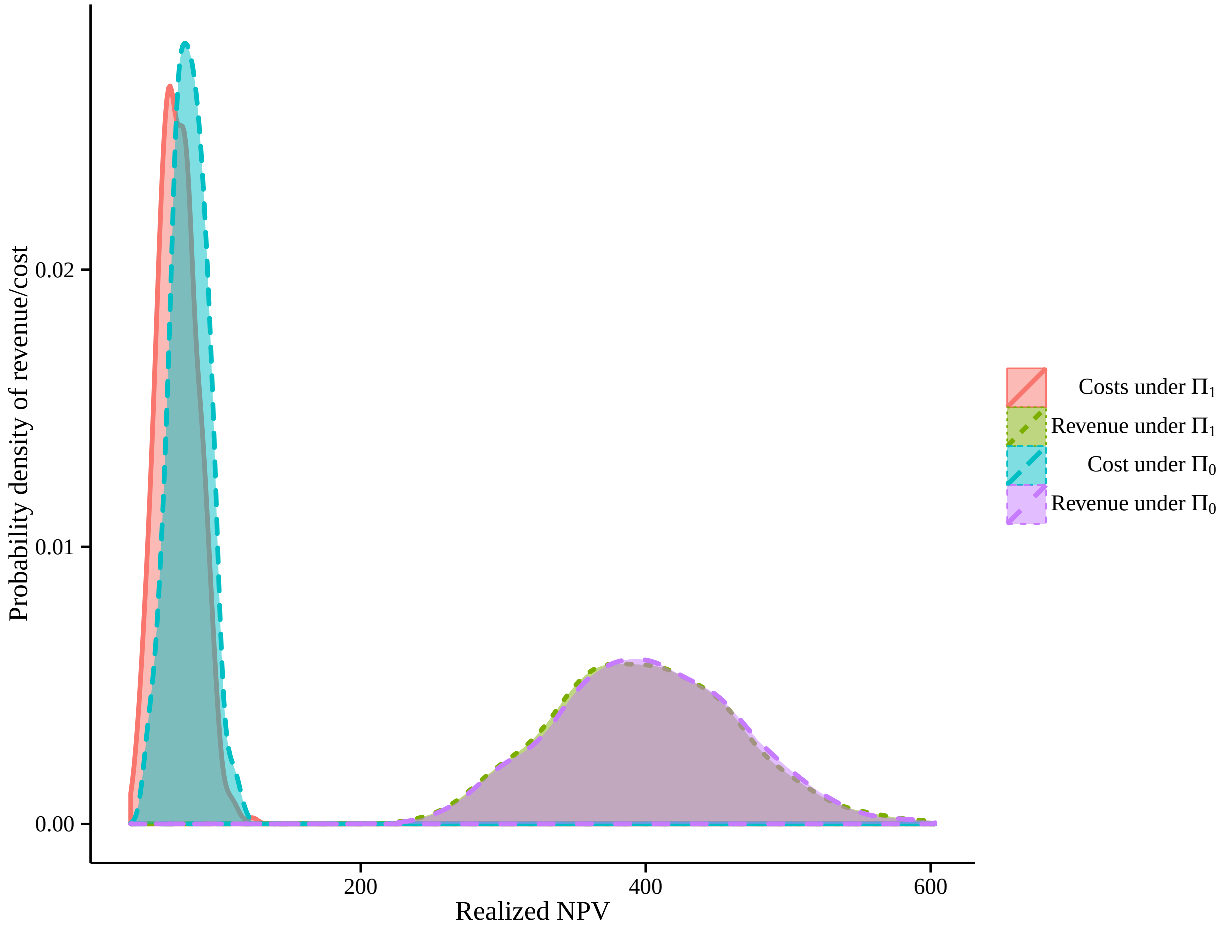


Figure S10: Results as in Figure 5 of the main text, but using a net reduction of NPV equal to 10%.

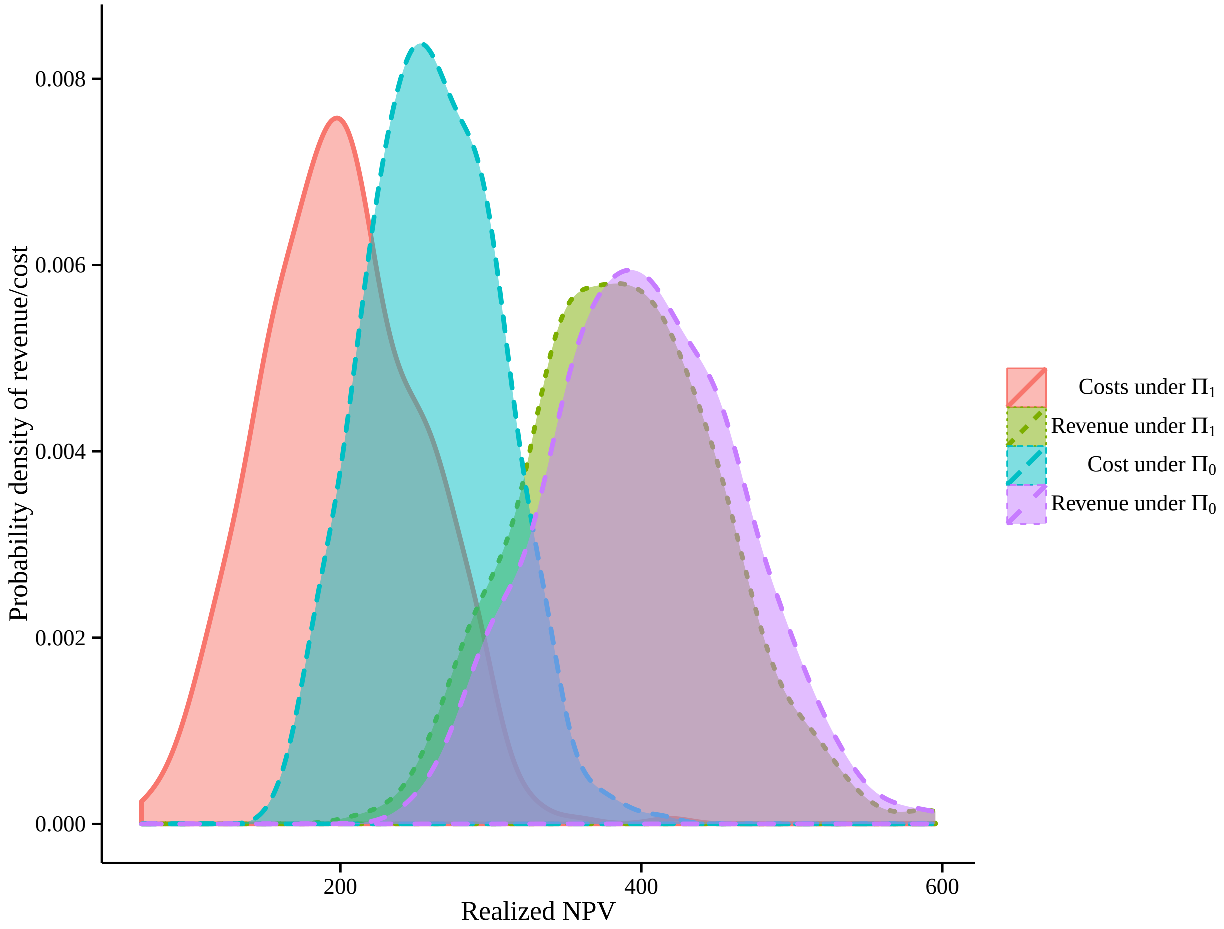


Figure S11: Results as in Figure 5, but using a net reduction equal to 30%
